# Supplementary material for: De-fine: Decomposing and Refining Visual Programs with Auto-Feedback
Source: arXiv:2311.12890 source file (2024-08-05)
Supplement: Supplementary file 1 [file Supplementary_Material_2472.pdf]

# A PSEUDOCODE DIAGRAM

We show a pseudocode algorithm here so that readers can better understand our process in Figure 2.

**Algorithm 1:** The algorithm of **De-fine**

**Input:** An image $x$ and a query $q$
**Output:** The *result* of the query $q$ about image $x$

Logic_step = LLM_decompose($q$);
Abstract_code = sketch($c$ in *codebase* if $c$.comments() relevant to $q$);
AL = Logic_step, Abstract_code;
**for** *i in iteration* **do**
    Origin_code = Code_generator(API,AL,$q$);
    Feedback = Feeback_generator(Compilor(Origin_code,$x$));
    Code = Refiner(Origin_code,Feedback);
**end**
result = Compilor(Code,x)

# B THE IMPACT OF CAPTION AND INFORMATION

The improvements in performance are not solely due to providing captions or information for images. In the appendix, we conducted additional ablation experiments on the backbone, where the backbone was only given the captions of images and the textual traces after code execution. Comparing this data to our results in Table 5, there remains a noticeable difference. This indicates that it is our feedback mechanism, rather than the addition of information, that contributes to the performance improvements.

**Table 8: Evaluation of Caption and Information.**

| | GQA |
|---|---|
| Backbone | 52.6 |
| + caption | 53.7 |
| + execution trace | 52.8 |
| + compiler output | 52.6 |

# C HUMAN EVALUATION

In this section, we explain the sources of error details of our experiments in Figure 5. We manually selected 100 samples from the GQA dataset, analyzed each program's errors, and classified them into five categories: 1) Incorrect Program: For those programs that cannot be compiled, we all classify error codes. 2) Multiple Answer: As the function 'best_text_match' will return the most relevant string of image patch, there may be multiple correct results in the result. Therefore, the errors corresponding to this function are classified as Multiple Answer. 3) VQA: In the method, we have the 'simple_query' function, the 'llm_query' function and the 'verify_property' function. These question-and-answer functions correspond to the Vqa function of Visual Programming. The program errors caused by these functions will be classified as VQA. 4) Location: Positioning is very critical in visual tasks. It is implemented by the 'Loc' function in Visual Programming and the 'find' function in **De-fine**. 5) Crop: In Visual Programming, there is the 'Crop' function, while in **De-fine** it is defined in the 'ImagePatch' class. Therefore, incorrect answers due to image cropping will be recorded here.

# D PROMPT USED IN THE MODEL.

We used the following prompt during our experiments:

**Logical Step Decompose**:

```
Given a VQA query, output the decomposed sub-step to how to answer it.
The output must be brief and short.
Query: <QUERY>
Your answer should only start with #step1:, #step2 etc.:
```

**Code Generation**:

```
You are a helpful assistant.
<API>
<AL_PROMPT>
<QUERY>
Only answer with a function starting def execute_command(image):
```

**Visual Feedback (Image caption)**:

```
Please give me a short caption of <IMAGE2> located in the <BBOX> of <IMAGE1>.
It mainly focuses on the connection between the object itself and the overall picture:
```

**Visual Feedback (Sub-step verification)**:

```
<IMAGE_LIST> Is it possible that these pictures are the output of <substeps>?
```

**Textual Feedback (Text summarization)**:

```
<TRACE> Please summarize in natural language what program trace outputs.
```

**Textual Feedback (Logical verification)**:

```
<SUB_STEPS> Is it possible that these sub_steps can solve <QUERY>?
If not, please modify it and only start with #step1:, #step2 etc.:
```

**Refiner Prompt**:

```
You are a program optimizer (or corrector).

I will give you some information about how to use an API and a query about a picture.
Your task is to refine (or correct) the code that can answer the query by using API.
Please refine (or correct) the origin code based on feedbacks.

[API manual]: <API_MANUAL>
[Query]: <QUERY>
[Code]: <ORIGIN_CODE>
[Visual Feedback]: <FEEDBACK_V>
[Textal Feedback]: <FEEDBACK_T>
[Compile Feedback]: <FEEDBACK_C>
Your answer should start with:
def execute_command(image):
```

## E ERROR CASES

1) **On the GQA task**, for the image named n172618.jpg, with the question "What is the height of the girl that is holding the kite?", De-fine generated the following code:

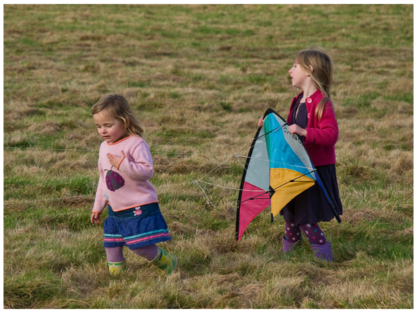

**Figure 7: Image n172618.jpg with query "What is the height of the girl that is holding the kite?"**

```
def execute_command(image):
    #Step1: Find the patch containing the girl
    girl_patches = ImagePatch(image).find("girl")
    #Step2: Find the girl holding the kite
    kite_patches = ImagePatch(image).find("kite")
    kite_patch = kite_patches[0]
    girl_holding_kite_patches = []
    for girl_patch in girl_patches:
        if girl_patch.overlaps_with(kite_patch.left, kite_patch.lower, kite_patch.right, kite_patch.upper):
            girl_holding_kite_patches.append(girl_patch)
    #Step3: Calculate the height of the girl holding the kite
    girl_holding_kite_patch = girl_holding_kite_patches[0]
    height = girl_holding_kite_patch.upper - girl_holding_kite_patch.lower
    return str(height) + "pixels"
```

**Listing 1: Code for image n172618.jpg**

Although the code is executed correctly and the logic was sound, the result was incorrect when compared to the expected answer "Tall". This is because the question could not be adequately transformed into a classification problem of tall or short.

2) **On the OK-VQA task**, regarding the image COCO_val2014_000000029393.jpg with the question, “What type of dog is this?”, De-fine produced the following code:

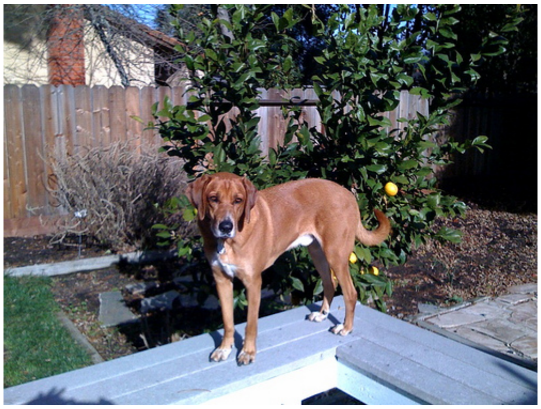

**Figure 8: Image COCO_val2014_000000029393.jpg with query “What type of dog is this?”**

```
def execute_command(image):
    #Step1: Create an ImagePatch object from the image
    image_patch = ImagePatch(image)
    #Step2: Use simple_query method to get the answer
    dog_breed = image_patch.simple_query("What type of dog is this?")
    #Step3: Return the answer
    return dog_breed
```

**Listing 2: Code for image COCO_val2014_000000029393.jpg**

The error in this instance was related to the use of the Blip tool in the simple_query function, which returned the answer "a dachshund". However, when we replaced the function called by simple_query with GPT-4V, "Rhodesian Ridgeback" was obtained. Although the label is "hound".

# F FEEDBACK GENERATOR OUTPUT EXAMPLE

Our feedback is multifaceted. We will showcase some examples from the experimental process and include them in the appendix:
1) **On the GQA task**, for the image named n172618.jpg, with the question “What is the height of the girl that is holding the kite?”, De-fine generated the following feedback:

**Visual Feeback**: The young girl on the right in vibrant outdoor clothing holds onto a colorful kite, preparing to catch the wind on a lively day in the field. The young adventurer on the left in a pink sweater encounters the wonders of nature and the images you've provided do seem like they could be the result of an operation that extracts a specific area or "patch" from a larger image

**Textual Feeback**: There is a kite. There is a child holding the kite in her hand. The height of the child holding the kite is 355 pixels. Those sub-steps could be part of a process to estimate the height of the girl holding the kite.

**Compile Feeback**: Execution succeed!

2) **On the OK-VQA task**, regarding the image COCO_val2014_000000029393.jpg with the question, “What type of dog is this?”, De-fine generated the following feedback:

**Visual Feeback**: A vigilant dog stands guard on a sunlit garden deck, with a lemon tree backdrop. From the context provided, it seems like these images could indeed be part of such a picture.

**Textual Feeback**: The breed of the dog is dachshund. But those steps alone are insufficient to determine the breed of a dog from an image. A specialized image recognition model would be required.

**Compile Feeback**: Execution succeed!

# G CODE GENERATED BY DIFFERENT ENGINES

In this section, we show the program output by different code generation engines and try to analyze them. Specifically, we take the same prompt as input and generate the corresponding codes by Code-Llama (34B), Code-Llama (70B), and GPT-3.5-Turbo (1106) respectively. In the subsequent exposition, we present a trio of illustrative examples involving multi-step queries and their corresponding responses, wherein the generation of code was efficaciously accomplished notwithstanding the limitations inherent in the model. Nevertheless, it is pertinent to acknowledge that the Code-Llama (70B) model exhibits occasional discrepancies in its interpretation of the ‘verify_property’

function. Concurrently, the Code-Llama (34B) variant demonstrates a partial deficiency in its capacity to decompose the problem at hand, potentially leading to lapses in logical reasoning.

**Query: Does the flag that is to the left of the bucket have large size and blue color?**

```python
def execute_command(image):
    #Step1: Find the flag and bucket patches
    flag_patches = ImagePatch(image).find("flag")
    bucket_patches = ImagePatch(image).find("bucket")
    #Step2: Check if there is a flag to the left of the bucket
    for flag_patch in flag_patches:
        if flag_patch.horizontal_center < bucket_patches[0].horizontal_center:
            #Step3: Check if the flag has large size and blue color
            if flag_patch.verify_property("flag", "large") and flag_patch.verify_property("flag", "blue"):
                return "yes"
    #Step4: If no flag to the left of the bucket has large size and blue color, return "no"
    return "no"
```

**Listing 3: Python program generated by GPT-3.5-Turbo (1106)**

```python
def execute_command(image):
    #Step1: Find the bucket and flag patches
    image_patch = ImagePatch(image)
    bucket_patches = image_patch.find("bucket")
    flag_patches = image_patch.find("flag")
    #Step2: Check if there is a flag to the left of the bucket
    flag_patches_left = []
    for flag_patch in flag_patches:
        for bucket_patch in bucket_patches:
            #Step3: Check if the flag has large size and blue color
            if flag_patch.left > bucket_patch.left and flag_patch.right < bucket_patch.right:
                flag_patches_left.append(flag_patch)
    if len(flag_patches_left) == 0:
        return "no"
    #Step4: Return if flag to the left of the bucket has large size and blue color
    flag_patch = flag_patches_left[0]
    return bool_to_yesno(flag_patch.verify_property("flag", "size", "large") and flag_patch.verify_property("flag", "color", "blue"))
```

**Listing 4: Python program generated by Code-Llama (70B)**

```python
def execute_command(image):
    #Step1: Find the flag and bucket patches
    image_patch = ImagePatch(image)
    flag_patches = image_patch.find("flag")
    bucket_patches = image_patch.find("bucket")
    flag_patch = flag_patches[0]
    bucket_patch = bucket_patches[0]
    #Step2: Return if flag to the left of the bucket has large size and blue color
    return bool_to_yesno(flag_patch.verify_property("flag", "large") and flag_patch.verify_property("flag", "blue") and flag_patch.
      verify_property("flag", "left", bucket_patch))
```

**Listing 5: Python program generated by Code-Llama (34B)**

**Query: Of what race is the man the skateboard is to the right of?**

```python
def execute_command(image):
    # Step1: Find the man patch
    image_patch = ImagePatch(image)
    man_patches = image_patch.find("man")
    man_patch = man_patches[0]
    # Step2: Find the skateboard patch to the right of the man
    skateboard_patches = image_patch.find("skateboard")
    right_skateboard_patches = []
    for skateboard_patch in skateboard_patches:
        if skateboard_patch.left > man_patch.right:
            right_skateboard_patches.append(skateboard_patch)
    # Step3: Find the race of the man the skateboard is to the right of
    race = ""
    if len(right_skateboard_patches) > 0:
        race = right_skateboard_patches[0].simple_query("What is the race of the man?")
    return race
```

**Listing 6: Python program generated by GPT-3.5-Turbo (1106)**

```python
def execute_command(image):
    # Step1: Find the skateboard patch
    image_patch = ImagePatch(image)
    skateboard_patches = image_patch.find("skateboard")
    skateboard_patch = skateboard_patches[0]
    # Step2: Find the man the skateboard is to the right of
    man_patches = image_patch.find("man")
    for man_patch in man_patches:
        if man_patch.right > skateboard_patch.right:
            # Step3: Return the race of the man
            return man_patch.simple_query("What race is this man?")
```

**Listing 7: Python program generated by Code-Llama (70B)**

```python
def execute_command(image):
    # Step1: Find the skateboard patch
    image_patch = ImagePatch(image)
    skateboard_patches = image_patch.find("skateboard")
    skateboard_patch = skateboard_patches[0]
    # Step2: Find the man patch
    man_patches = image_patch.find("man")
    man_patch = man_patches[0]
    # Step3: Return the race of the man the skateboard is to the right of
    if skateboard_patch.horizontal_center > man_patch.horizontal_center:
        return man_patch.simple_query("What is the race of the man?")
    else:
        return "No man in the image"
```

**Listing 8: Python program generated by Code-Llama (34B)**

**Query: Is the material of the computer monitor the same as the TV?**

```python
def execute_command(image):
    # Step1: Find the patches for the computer monitor and the TV
    image_patch = ImagePatch(image)
    monitor_patches = image_patch.find("computer monitor")
    tv_patches = image_patch.find("TV")
    # Step2: Check if the material of the computer monitor is the same as the TV
    monitor_material = monitor_patches[0].simple_query("What is the material?")
    tv_material = tv_patches[0].simple_query("What is the material?")
    is_same_material = monitor_material == tv_material
    # Step3: Return the answer
    return bool_to_yesno(is_same_material)
```

**Listing 9: Python program generated by GPT-3.5-Turbo (1106)**

```python
def execute_command(image):
    # Step1: Find the computer monitor patches
    image_patch = ImagePatch(image)
    computer_patches = image_patch.find("computer monitor")
    # Step2: Check if the material of the computer monitor is the same as the TV
    tv_patches = image_patch.find("tv")
    for computer_patch in computer_patches:
        for tv_patch in tv_patches:
            if computer_patch.overlaps_with(tv_patch):
                # Step3: Return the answer
                return bool_to_yesno(computer_patch.verify_property(tv_patch)
```

**Listing 10: Python program generated by Code-Llama (70B)**

```python
def execute_command(image):
    # Step1: Find the computer monitor and TV patches
    image_patch = ImagePatch(image)
    computer_monitor_patches = image_patch.find("computer monitor")
    tv_patches = image_patch.find("TV")
    # Step2: Check if the material of the TV is the same as the computer monitor
    tv_patch = tv_patches[0]
    computer_monitor_patch = computer_monitor_patches[0]
    return bool_to_yesno(tv_patch.verify_property("TV", "material") == computer_monitor_patch.verify_property("computer monitor", "material"))
```

**Listing 11: Python program generated by Code-Llama (34B)**
